# Supplementary material for: Differentiable Trust Region Layers for Deep Reinforcement Learning
Source: arXiv:2101.09207 source file (2021-03-09)
Supplement: Supplementary file 1 [file derivations.tex]

\documentclass{article}

% if you need to pass options to natbib, use, e.g.:
%     \PassOptionsToPackage{numbers, compress}{natbib}
% before loading neurips_2020

% ready for submission
% \usepackage{neurips_2020}

% to compile a preprint version, e.g., for submission to arXiv, add add the
% [preprint] option:
%     \usepackage[preprint]{neurips_2020}

% to compile a camera-ready version, add the [final] option, e.g.:
%     \usepackage[final]{neurips_2020}

% to avoid loading the natbib package, add option nonatbib:
%  \usepackage[nonatbib]{neurips_2020}

\usepackage[utf8]{inputenc} % allow utf-8 input
\usepackage[T1]{fontenc}    % use 8-bit T1 fonts
\usepackage{hyperref}       % hyperlinks
\usepackage{url}            % simple URL typesetting
\usepackage{booktabs}       % professional-quality tables
\usepackage{amsfonts}       % blackboard math symbols
\usepackage{nicefrac}       % compact symbols for 1/2, etc.
\usepackage{microtype}      % microtypography

%%%%%%%%%%%%%%%%%%%%%%%%%%%%%%%%%%%%%%%%%%%%%%%%%%%%%%%%%%%%%%%%%%%%%%%%%%%%%%%%%%%%
% use it for comments
% TODO remove laterhttps://www.overleaf.com/project/5e42815f97cde100018a029f
\usepackage{xargs}                      % Use more than one optional parameter in a new commands
\usepackage[pdftex,dvipsnames]{xcolor}  % Coloured text etc.
\usepackage[colorinlistoftodos,prependcaption,textsize=tiny]{todonotes}
\newcommandx{\unsure}[2][1=]{\todo[linecolor=red,backgroundcolor=red!25,bordercolor=red,#1]{#2}}
\newcommandx{\change}[2][1=]{\todo[linecolor=blue,backgroundcolor=blue!25,bordercolor=blue,#1]{#2}}
\newcommandx{\info}[2][1=]{\todo[linecolor=OliveGreen,backgroundcolor=OliveGreen!25,bordercolor=OliveGreen,#1]{#2}}
\newcommandx{\improvement}[2][1=]{\todo[linecolor=Plum,backgroundcolor=Plum!25,bordercolor=Plum,#1]{#2}}
\newcommandx{\thiswillnotshow}[2][1=]{\todo[disable,#1]{#2}}

% ------------------------------------------------------------------------------
% Math stuff
% ------------------------------------------------------------------------------

\usepackage{mathtools}
\usepackage{bm}
\usepackage[short]{optidef}
\usepackage{nicefrac}       % compact symbols for 1/2, etc.

\DeclareMathOperator*{\argmax}{arg\,max}
\DeclareMathOperator*{\argmin}{arg\,min}

\newcommand{\KL}[2]{\textrm{KL}\left( {#1} \parallel {#2} \right)}
\newcommand{\st}{\textrm{s.t.}}
\newcommand{\old}[1]{{#1}_{\textrm{old}}}
\newcommand{\til}[1]{\tilde{#1}}

\newcommand{\nf}[2]{{\frac{#1}{#2}}}
\newcommand{\nff}{^{\nicefrac{1}{2}}}
\newcommand{\tr}[1]{\mathrm{tr}\left(#1\right)}

\title{Information Theoretic Constraints with Convex Optimization Layers}
\author{Fabian~Otto \\
  Bosch Center for Artificial Intelligence, Eberhard Karls Universität Tübingen\\
  \texttt{fabian.otto@de.bosch.com}
\And Gerhard~Neumann,
\And Philipp~Becker
}

% The \author macro works with any number of authors. There are two commands
% used to separate the names and addresses of multiple authors: \And and \AND.
%
% Using \And between authors leaves it to LaTeX to determine where to break the
% lines. Using \AND forces a line break at that point. So, if LaTeX puts 3 of 4
% authors names on the first line, and the last on the second line, try using
% \AND instead of \And before the third author name.

\author{%
  David S.~Hippocampus\thanks{Use footnote for providing further information
    about author (webpage, alternative address)---\emph{not} for acknowledging
    funding agencies.} \\
  Department of Computer Science\\
  Cranberry-Lemon University\\
  Pittsburgh, PA 15213 \\
  \texttt{hippo@cs.cranberry-lemon.edu} \\
}

\begin{document}

\maketitle

\begin{abstract}
  The abstract paragraph should be indented \nicefrac{1}{2}~inch (3~picas) on
  both the left- and right-hand margins. Use 10~point type, with a vertical
  spacing (leading) of 11~points.  The word \textbf{Abstract} must be centered,
  bold, and in point size 12. Two line spaces precede the abstract. The abstract
  must be limited to one paragraph.
\end{abstract}

\section{Information Theoretic Trust Regions using CVXPYLayers}
\subsection{Marginal Case}
Similar to information theoretic policy search algorithms \cite{Abdolmaleki2015}, we want to control the exploration-exploitation trade-off by bounding the relative entropy of two subsequent search distributions. However, by bounding the KL, the algorithm can adapt the mean and the variance of the algorithm. In order to maximize the objective for the immediate iteration, the shrinkage in the variance typically dominates the contribution to the KL-divergence, which often leads to a premature convergence of these algorithms. Hence, in addition to control the KL-divergence of the update, we also need to control the shrinkage of the covariance matrix. Such a control mechanism can be implemented by lower-bounding the entropy of the new distribution.

Finding a new search distribution $q^*(x)$ in this setting can be achieved by solving the following optimization problem
\begin{equation}
    q^*(x) = \underset{q}{\argmax} \int q(x) R(x) dx\quad \st \quad \KL{q(x)}{\old{q}(x)} \leq \epsilon, \quad \textrm{H}\left(\til{q}(x) \right) \geq \beta
\end{equation}
In the strictly Gaussian case a policy update in closed form can be formulated \cite{Peters2010}. 
For this work, we extend this setting to arbitrary distributions as well as to the deep setting (Section~\ref{sec:deep}) by leveraging differentiable convex optimization layers \cite{Agrawal2019}.
For the marginal case, the original optimization objective simplifies to \improvement{This might be wrong.} 
\begin{equation}
    q^*(x) = \underset{q(x)}{\argmax} \int q(x) R(x) dx,
\end{equation}
The optimization layer, however, is solving the following optimization problem
\begin{equation}
    \underset{\til{q}(x)}{\argmin}  \quad d\left(q(x), \til{q}(x) \right) \quad \text{s.t.} \quad \KL{\til{q}(x)}{\old{q}(x)} < \epsilon, \quad \textrm{H}\left(\til{q}(x) \right) > \beta,
\end{equation}
where $\til{q}(x)$ is the projected output of the optimization layer and $d(\cdot, \cdot)$ represents a similarity measure, e.\,g. the Euclidean distance $d(x, y) = ||x-y||^2_2$ or KL-divergence $d(x, y) = KL(x||y)$.
\improvement{Currently I do not know how to use the KL in this layer for the parameters. The required DPP formulation might not allow to do that.}
Lastly, $\old{q}(x) = \til{q}^*(x)$ represents the projected distribution from the previous iteration. 
In this simple case, where $q(x)$ represents a parametric distribution, the projected parameters from $\til{q}(x)$ can be assigned to $q(x)$, this allows to modifiy the gradient during learning based on the optimization layer. 

Possible experiments in this setting in include mainly stochastic search cases, e.\,g. Rosenbrock or similar. 
\improvement{I am currently not sure which ones to add. Bentcigar and Ellipsoide might be good additional options.}
Experiments are planned for two scenarios
\begin{itemize}
    \item White box function, i.\,e. gradient is accessible. This typically enables us evaluate the function without significant cost, consequently sample performance is not relevant. Further, we can reparametrize the Gaussian output of the projection layer to update the policy $q(x)$: 
        \begin{align}
        \nabla_{q} R(g(\mu, \Sigma, \epsilon)) \qquad\qquad \epsilon \sim \mathcal{N}(0, I), 
        \end{align}
    \item Black box function, i.\,e. gradient is not accessible. This makes sample performance in most cases highly relevant, because either simulation or real environment have higher computational costs. In this setting importance sampling can be used to update the policy as
    \begin{equation}
        \nabla_{q} \nf{\til{q}(x)}{\old{q}(x)} R(x) - B(x),
    \end{equation}
    where $B(x)$ represents a baseline.
\end{itemize}
Comparisons should be conducted against MORE \cite{Abdolmaleki2015}, REPS \cite{Peters2010} and PAPI \cite{Akrour2019}. 
Furthermore, leveraging PPO \cite{Schulman2017} and TRPO \cite{Schulman2015} for the importance sampling objective seem to be most reasonable. 
Interesting points would be to see KL and Entropy progress as well as convergence and final performance (reward \& samples). 

% \begin{itemize}
%     \item Subsequent CVXPYLayer 
%     $$ \underset{\til{q}(x)}{\textrm{argmin}}  \quad d\left(q(x), \til{q}(x) \right) \quad \text{s.t.} \quad \KL{\til{q}(x)}{\old{q}(x)} < \epsilon, \quad \textrm{H}\left(\til{q}(x) \right) > \beta $$
%     \item optimize $\til{q}^*(x) = \underset{\til{q}(x)}{\textrm{argmax}} \int \til{q}(x) R(x) dx$
%     \item $\old{q}(x) = \til{q}^*(x)$
% \end{itemize}
% Applications:
% \begin{itemize}
%     \item Stochastic Search (Better than PAPI? Which (according to PAPI paper better than MORE and REPS?)
%     \item Closed form solutions no longer available (Flows, Factor Analyzers ... )
% \end{itemize}

\subsection{Deep Projections}
\label{sec:deep}
For the deep RL case, the policy $q(x|y)$ is conditioned on some context $y$ and modelled by a neural network. 
This also changes the optimization layer to 
\begin{equation}
    \til{q}^*(x | y) = \underset{\til{q}(x | y)}{\argmin}  \quad d\left(q(x|y), \til{q}(x|y) \right) \quad \st \quad \KL{q(x|y)}{\old{q}(x|y)} \leq \epsilon, \quad \textrm{H}\left(q(x|y) \right) \geq \beta
\end{equation}
In this setting $d\left(q(x|y), \til{q}(x|y) \right)$ represents the difference of the output distributions for each sample. 
This means the solution will lead to a projected predictive distribution for each sample. 
However, this makes the above marginal setting no longer viable. 
Assigning specific outputs to neural networks is not directly possible, therefore it is required to either 
\begin{enumerate}
    \item use the optimization layer during inference,
    \item conduct an additional regression step after $n$ update steps,
    \item or optimize environment and regression objective at the same time.
\end{enumerate}
For the latter we can introduce an separate loss in the objective.
\begin{equation}
    q^*(x | y) = \underset{q(x|y)}{\argmax} \int q(y) \int q(x|y) R(x,y) dx - \alpha  d\left(q(x|y), \til{q}^*(x | y)\right) dy
\end{equation}
A drawback of this approach is, we lose all guarantees from the first case, any prediction might satisfy the constraints or not. 
On the other hand, unlike existing methods, this allows to constrain each context/state individually, while the projection affects the whole network and not only the last layer. 
More specifically, the above formulation only penalizes the loss in case the bounds are violated. 
Otherwise, the similarity measure $d(\cdot, \cdot)$ and gradient will be $0$, assuming suitable $d$.

Regarding experiments, PAPI \cite{Akrour2019}, PPO \cite{Schulman2017} and TRPO \cite{Schulman2015} should be evaluated on different contextual task. 
Maybe any robot tasks or standard Mujoco environments should be fine. 
Currently, the layers are quite slow, therefore, choosing smaller environments, which converge faster and require smaller amounts of samples is preferred. 

% \begin{itemize}
%     \item Conditional Distribution / Policy 
%     \item Subsequent CVXPYLayer 
%     $$ \til{q}^*(x | y) = \underset{\til{q}(x | y)}{\textrm{argmin}}  \quad d\left(q(x|y), \til{q}(x|y) \right) \quad \text{s.t.} \quad \KL{q(x|y)}{\old{q}(x|y)} < \epsilon, \quad \textrm{H}\left(q(x|y) \right) > \beta $$
%   \item Optimize
% $$  \underset{q(x|y)}{\textrm{argmax}} \int q(y) \int q(x|y) R(x,y) dx - \alpha  d\left(q(x|y), \til{q}^*(x | y)\right) dy $$
% \end{itemize}
% Benefits:
% \begin{itemize}
%     \item Constraints per context/state, no expectation
%     \item Exact Projection
%     \item Projection affects the whole network by backpropagation not just last layer
%     \item Penalty term (and gradient) 0 as long as $q$ is inside of trust region (for reasonable $d$)
% \end{itemize}

\section{Derivations}
\subsection{Mean}
\begin{align}
    L(\lambda) &= \left(\frac{\tilde{\mu} + \lambda\mu_{old}}{1+\lambda} - \tilde{\mu}\right)^T\Sigma^{-1}\left(\frac{\tilde{\mu} + \lambda\mu_{old}}{1+\lambda} - \tilde{\mu}\right) +\\
    &+\lambda \left(\left(\frac{\tilde{\mu} + \lambda\mu_{old}}{1+\lambda} - \mu_{old}\right)^T\Sigma^{-1}\left(\frac{\tilde{\mu} + \lambda\mu_{old}}{1+\lambda} - \mu_{old}\right) - \epsilon\right) \\
   & =k \frac{\lambda^2}{(1+\lambda)^2}  + k \frac{\lambda}{(1+\lambda)^2} -\lambda \epsilon \\
\end{align}
where $
k =  \left(\tilde{\mu} -\mu_{old}\right)^T\Sigma^{-1} \left(\tilde{\mu} -\mu_{old}\right)$

Thus,
\begin{align}
  \frac{\partial }{\partial\lambda} L(\lambda) &= \frac{k} {(1+\lambda)^2} - \epsilon  
\end{align}

So, $$
\lambda = \sqrt{\frac{k}{\epsilon}}-1 =  \sqrt{\frac{\left(\tilde{\mu} -\mu_{old}\right)^T\Sigma^{-1} \left(\tilde{\mu} -\mu_{old}\right)}{\epsilon}}-1
$$

\subsection{Mean linear}

\begin{align}
    &\argmin_{\mu}~ (\mu - \old{\mu})^T (\til{\mu} - \old{\mu})\\
    &\st ~(\mu - \old{\mu})^T \Sigma^{-1} (\mu - \old{\mu}) \leq \epsilon,
\end{align}

\subsubsection{Dual}

In the following: $c = \til{\mu}-\old{\mu}$
\begin{align}
    L(\mu, \lambda) &= \mu^Tc - \old{\mu}^Tc + \lambda(\epsilon - \mu^T\Sigma^{-1}\mu +2\mu^T\Sigma^{-1}\old{\mu} - \old{\mu}^T\Sigma^{-1}\old{\mu}) \\
    \nf{\partial L}{\partial\mu} &= c - 2\lambda \Sigma^{-1}\mu +2\lambda\Sigma^{-1}\old{\mu}\\
    \rightarrow \mu^*&= \Sigma\nf{c+2\lambda\Sigma^{-1}\old{\mu}}{2\lambda}\\
                     &= 0.5*\lambda^{-1}\Sigma c +\old{\mu}
\end{align}
\subsubsection{Primal}
\begin{align}
    \nf{\partial\mu}{\partial\lambda} &= -0.5\lambda^{-2}\Sigma c  \\
    \nf{d(\mu^T\Sigma^{-1}\mu)}{d\lambda} &= \nf{\partial(0.5*\lambda^{-1} c^T +\old{\mu}^T\Sigma^{-1})(0.5*\lambda^{-1}\Sigma c +\old{\mu})}{\partial\lambda} \\
    &= \nf{\partial(0.25*\lambda^{-2} c^T \Sigma c + \lambda^{-1}\old{\mu}^Tc +\mu^T_{old}\Sigma^{-1}\old{\mu})}{\partial\lambda}\\
    &= -0.5*\lambda^{-3} c^T \Sigma c - \lambda^{-2}\old{\mu}^Tc \\
    \nf{\partial (2\mu^T\Sigma^{-1}\old{\mu})}{\partial\lambda} &= \nf{\partial(\lambda^{-1}c^T\old{\mu})}{\partial\lambda} = -\lambda^{-2}c^T\old{\mu}
\end{align}

\begin{align}
    \nf{\partial L(\mu^*, \lambda)}{\partial\lambda} &= -0.5\lambda^{-2}c^T\Sigma c + \epsilon - 0.25*\lambda^{-2} c^T \Sigma c - \lambda^{-1}\old{\mu}^Tc -\mu^T_{old}\Sigma^{-1}\old{\mu} + \\
    &\lambda^{-1} c^T\old{\mu} +\old{\mu}^T\Sigma^{-1}\old{\mu} 
   +0.5*\lambda^{-2} c^T \Sigma c + \lambda^{-1}\old{\mu}^Tc -\lambda^{-1}c^T\old{\mu}
\end{align}

\begin{align}
    \nf{\partial L(\mu^*, \lambda)}{d\lambda} &=  \epsilon - 0.25*\lambda^{-2} c^T \Sigma c \\
    \lambda^{-2} &= 4 * \epsilon (c ^T \Sigma c)^{-1}\\
    \lambda^* &= \pm \sqrt{\nf{1}{4 * \epsilon (c ^T \Sigma c)^{-1}}}\\
    \lambda^* &= \pm \sqrt{\nf{(c ^T \Sigma c)}{4 * \epsilon}}\\
    \longrightarrow \mu^* &= 0.5 \sqrt{\nf{(c ^T \Sigma c)}{4\epsilon}}^{-1}\Sigma c +\old{\mu}\\
    &= \sqrt{\nf{\epsilon}{(c ^T \Sigma c)}}\Sigma c +\old{\mu}
\end{align}

% \begin{align}
%     \mu^* &= \nf{2\lambda \old{\mu}^T + \old{\mu}^T\Sigma - \til{\mu}^T\Sigma}{2\lambda}  \\
%     \nf{dL}{d\mu} &= 2\lambda \Sigma^{-1}(\mu - \old{\mu}) -\old{\mu} + \til{\mu}\\
%     \nf{d\mu}{d\lambda} &= \nf{-\Sigma\old{\mu} + \Sigma\til{\mu}}{2\lambda^2}
%     \nf{dL(\mu^*, \lambda)}{d\lambda} = -0.5\lambda^{-2}c^T\Sigma c 
% \end{align}

\subsection{Variance 0} 
\begin{align}
    &\argmin_{\Sigma}~ \textrm{trace}\big((\Sigma - \old{\Sigma})^T (\til{\Sigma} - \old{\Sigma}) \big)\\
    &\st ~ \textrm{trace}(\old{\Sigma}^{-1} \Sigma) + k + \log|\old{\Sigma}| - \log|\Sigma| \leq \epsilon,
\end{align}

\subsubsection{Dual}
\begin{align}
    &\nf{\partial L}{\partial \Sigma} = \til{\Sigma} - \old{\Sigma} + \lambda \old{\Sigma}^{-1} - \lambda \Sigma^{-1} \\
    &\rightarrow \Sigma^* = \lambda \left(\lambda \old{\Sigma}^{-1} - \til{\Sigma} + \old{\Sigma} \right)^{-1}
\end{align}

\subsubsection{Primal}
\begin{align}
    \nf{\partial\Sigma^*}{\partial \lambda} &=  \textrm{trace}\left( \til{\Sigma} \nf{\partial \Sigma^*}{\partial \lambda}\right) - \textrm{trace}\left( \old{\Sigma} \nf{\partial \Sigma^*}{\partial \lambda} \right) +\lambda \textrm{trace}\left( \old{\Sigma}^{-1} \nf{\partial \Sigma^*}{\partial \lambda} \right)
    - \lambda \textrm{trace}\left( \nf{\til{\Sigma} - \old{\Sigma} +\lambda \old{\Sigma}^{-1}}{\lambda} \nf{\partial \Sigma^*}{\partial \lambda}\right)\\
    &+\textrm{trace}(\old{\Sigma}^{-1} \lambda \left(\lambda \old{\Sigma}^{-1} - \til{\Sigma} + \old{\Sigma} \right)^{-1}) + k + \log|\old{\Sigma}| - \log|\lambda \left(\lambda \old{\Sigma}^{-1} - \til{\Sigma} + \old{\Sigma} \right)^{-1}| - 2\epsilon\\
    &= \textrm{trace}(\old{\Sigma}^{-1} \lambda \left(\lambda \old{\Sigma}^{-1} - \til{\Sigma} + \old{\Sigma} \right)^{-1}) + k + \log|\old{\Sigma}| + k\lambda - \log| \left(\lambda \old{\Sigma}^{-1} - \til{\Sigma} + \old{\Sigma} \right)^{-1}| - 2\epsilon
\end{align}

\subsection{Variance 1} 
\begin{align}
    &\argmin_{\Sigma}~ \textrm{trace}(\til{\Sigma}^{-1} \Sigma) + k + \log|\til{\Sigma}| - \log|\Sigma|\\
    &\st ~ \textrm{trace}(\old{\Sigma}^{-1} \Sigma) + k + \log|\old{\Sigma}| - \log|\Sigma| \leq \epsilon,
\end{align}

\subsubsection{Dual}
\begin{align}
    &\nf{\partial L}{\partial \Sigma} = \til{\Sigma}^{-1} - \Sigma^{-1} - \lambda \old{\Sigma}^{-1} + \lambda \Sigma^{-1} \\
    & \rightarrow \Sigma^* = (\lambda -1) \left(\lambda \old{\Sigma}^{-1} - \til{\Sigma}^{-1} \right)^{-1}
\end{align}

\subsubsection{Primal}
\begin{align}
    \nf{\partial\Sigma^*}{\partial \lambda} &= \left(\lambda \old{\Sigma}^{-1} - \til{\Sigma}^{-1} \right)^{-1} + (\lambda -1) \left(-\lambda \old{\Sigma}^{-1} + \til{\Sigma}^{-1} \right)^{-2} \old{\Sigma}^{-1}\\
    &= \left(\til{\Sigma}^{-1} - \old{\Sigma}^{-1}\right) \left(\lambda \old{\Sigma}^{-1} - \til{\Sigma}^{-1} \right)^{-2}
\end{align}

\begin{align}
    \nf{\partial\old{\Sigma}^{-1} \Sigma^*}{\partial \lambda} &= \old{\Sigma}^{-1}\left(\lambda \old{\Sigma}^{-1} - \til{\Sigma}^{-1} \right)^{-1} + \old{\Sigma}^{-1}(\lambda -1) \left(-\lambda \old{\Sigma}^{-1} + \til{\Sigma}^{-1} \right)^{-2} \old{\Sigma}^{-1}\\
    &= \old{\Sigma}^{-1}\left(\til{\Sigma}^{-1} - \old{\Sigma}^{-1}\right) \left(\lambda \old{\Sigma}^{-1} - \til{\Sigma}^{-1} \right)^{-2}\\
    \nf{\partial \textrm{trace}\left(\old{\Sigma}^{-1}\Sigma^*\right)}{\partial \lambda} &= \textrm{trace}\left(\old{\Sigma}^{-1}\left(\til{\Sigma}^{-1} - \old{\Sigma}^{-1}\right) \left(\lambda \old{\Sigma}^{-1} - \til{\Sigma}^{-1} \right)^{-2}\right)
\end{align}

\begin{align}
    \nf{\partial L}{ \partial \lambda} &= \textrm{trace}\left(\til{\Sigma}^{-1}\left(\til{\Sigma}^{-1} - \old{\Sigma}^{-1}\right) \left(\lambda \old{\Sigma}^{-1} - \til{\Sigma}^{-1} \right)^{-2}\right)-\\
    &\textrm{trace}\left(\nf{\lambda \old{\Sigma}^{-1} - \til{\Sigma}^{-1}}{(\lambda -1)} \left(\til{\Sigma}^{-1} - \old{\Sigma}^{-1}\right) \left(\lambda \old{\Sigma}^{-1} - \til{\Sigma}^{-1} \right)^{-2}\right)+\\
    &\lambda \textrm{trace}\left(\old{\Sigma}^{-1}\left(\til{\Sigma}^{-1} - \old{\Sigma}^{-1}\right) \left(\lambda \old{\Sigma}^{-1} - \til{\Sigma}^{-1} \right)^{-2}\right) + \\
    & \lambda\textrm{trace}\left(\nf{\lambda \old{\Sigma}^{-1} - \til{\Sigma}^{-1}}{(\lambda -1)}\left(\til{\Sigma}^{-1} - \old{\Sigma}^{-1}\right) \left(\lambda \old{\Sigma}^{-1} - \til{\Sigma}^{-1} \right)^{-2}\right) - \\
    &\textrm{trace}\left(\old{\Sigma}^{-1} (\lambda -1) \left(\lambda \old{\Sigma}^{-1} - \til{\Sigma}^{-1} \right)^{-1}\right) - \\
    &k - \log|\old{\Sigma}| + \log|(\lambda -1) \left(\lambda \old{\Sigma}^{-1} - \til{\Sigma}^{-1} \right)^{-1}|  + \epsilon + \epsilon
\end{align}

\begin{align}
    &= \textrm{trace}\left(\til{\Sigma}^{-1}\left(\til{\Sigma}^{-1} - \old{\Sigma}^{-1}\right) \left(\lambda \old{\Sigma}^{-1} - \til{\Sigma}^{-1} \right)^{-2}\right)-\\
    &\lambda \textrm{trace}\left(\old{\Sigma}^{-1}\left(\til{\Sigma}^{-1} - \old{\Sigma}^{-1}\right) \left(\lambda \old{\Sigma}^{-1} - \til{\Sigma}^{-1} \right)^{-2}\right) + \\
    & \textrm{trace}\left(\left(\til{\Sigma}^{-1} - \old{\Sigma}^{-1}\right) \left(\lambda \old{\Sigma}^{-1} - \til{\Sigma}^{-1} \right)^{-1}\right) - \\
    &\textrm{trace}\left(\old{\Sigma}^{-1} (\lambda -1) \left(\lambda \old{\Sigma}^{-1} - \til{\Sigma}^{-1} \right)^{-1}\right) - \\
    &k - \log|\old{\Sigma}| + \log|(\lambda -1) \left(\lambda \old{\Sigma}^{-1} - \til{\Sigma}^{-1} \right)^{-1}|  + 2\epsilon
\end{align}

\begin{align}
    &= \textrm{trace}\left(\til{\Sigma}^{-1}\left(\til{\Sigma}^{-1} - \old{\Sigma}^{-1}\right) \left(\lambda \old{\Sigma}^{-1} - \til{\Sigma}^{-1} \right)^{-2}\right)-\\
    &\lambda \textrm{trace}\left(\old{\Sigma}^{-1}\left(\til{\Sigma}^{-1} - \old{\Sigma}^{-1}\right) \left(\lambda \old{\Sigma}^{-1} - \til{\Sigma}^{-1} \right)^{-2}\right) + \\
    & \textrm{trace}\left(\left(\til{\Sigma}^{-1} - \lambda\old{\Sigma}^{-1}\right) \left(\lambda \old{\Sigma}^{-1} - \til{\Sigma}^{-1} \right)^{-1}\right) - \\
    &k - \log|\old{\Sigma}| + \log|(\lambda -1) \left(\lambda \old{\Sigma}^{-1} - \til{\Sigma}^{-1} \right)^{-1}|  + 2\epsilon
\end{align}

\begin{align}
    &= \textrm{trace}\left(\til{\Sigma}^{-1}\left(\til{\Sigma}^{-1} - \old{\Sigma}^{-1}\right) \left(\lambda \old{\Sigma}^{-1} - \til{\Sigma}^{-1} \right)^{-2}\right)-\\
    &\lambda \textrm{trace}\left(\old{\Sigma}^{-1}\left(\til{\Sigma}^{-1} - \old{\Sigma}^{-1}\right) \left(\lambda \old{\Sigma}^{-1} - \til{\Sigma}^{-1} \right)^{-2}\right) - \\
    &2k - \log|\old{\Sigma}| + \log|(\lambda -1) \left(\lambda \old{\Sigma}^{-1} - \til{\Sigma}^{-1} \right)^{-1}|  + 2\epsilon
\end{align}

\begin{align}
    &= \textrm{trace}\left(\left(\til{\Sigma}^{-1}-\lambda\old{\Sigma}^{-1}\right)\left(\til{\Sigma}^{-1} - \old{\Sigma}^{-1}\right) \left(\lambda \old{\Sigma}^{-1} - \til{\Sigma}^{-1} \right)^{-2}\right)-\\
    &2k - \log|\old{\Sigma}| + \log|(\lambda -1) \left(\lambda \old{\Sigma}^{-1} - \til{\Sigma}^{-1} \right)^{-1}|  + 2\epsilon
\end{align}

\begin{align}
    &= \textrm{trace}\left(\left(\til{\Sigma}^{-1} - \old{\Sigma}^{-1}\right) \left(\lambda \old{\Sigma}^{-1} - \til{\Sigma}^{-1} \right)^{-1}\right)-\\
    &2k - \log|\old{\Sigma}| + \log|(\lambda -1) \left(\lambda \old{\Sigma}^{-1} - \til{\Sigma}^{-1} \right)^{-1}|  + 2\epsilon
\end{align}

\begin{align}
    &= \textrm{trace}\left(\left(\til{\Sigma}^{-1} - \old{\Sigma}^{-1}\right) \left(- \til{\Sigma} - \nf{(- \til{\Sigma})\lambda \old{\Sigma}^{-1}(- \til{\Sigma})}{1+ \lambda\textrm{trace}\left(\old{\Sigma}^{-1}(- \til{\Sigma})\right)} \right)\right)-\\
    &2k - \log|\old{\Sigma}| + k \log (\lambda -1) + \log| \left(\lambda \old{\Sigma}^{-1} - \til{\Sigma}^{-1} \right)^{-1}|  + 2\epsilon
\end{align}

rotation approach:
\begin{align}
&\Sigma = R^TD R
& B = R \sqrt(A) R^T
\end{align}

\begin{align}
&\nf{\partial \textrm{trace}(\sqrt A\sqrt{\Sigma})}{\partial \Sigma} = \nf{\partial\textrm{trace}(\sqrt A R^T \sqrt D R)}{\partial (R^T D R)}\\
&= \nf{\partial\textrm{trace}(\sqrt A R^T \sqrt D R)}{\partial D}\left(\nf{\partial D}{\partial \Sigma}\right)\\
\end{align}
\begin{align}
&\nf{\partial\textrm{trace}(B\sqrt{D})}{\partial D_{ab}}\\
&=\nf{\partial\sum_{ij}( B_{ij} \sqrt D_{ji} )}{\partial D_{ab}}\\
&=B_{ab}\odot\sqrt{D}_{ab}^{-1}\\
%    &= B_{aa}\odot\sqrt{D}_{aa}^{-1}
&= (R \sqrt A R^T)_{ab} \sqrt D_{ab}^{-1}\\
&= (\sum_{ij} R_{ai} \sqrt{A}_{ij} R_{jb}^T) \sqrt D_{ab}^{-1}\\
& = \sum_{ij} \sqrt{A}_{ij} R_{ja}^T\sqrt{D}_{ab}^{-1} R_{bi}
\end{align}

\begin{align}
&\nf{\partial\mathcal{L}}{\partial \Sigma} = (1 + \lambda)\mathrm{I}- (R \til{\Sigma}^{\nf{1}{2}} R^T)\odot D^{-\frac {1}{2}} - \lambda (R \old{\Sigma}^{\nf{1}{2}}R^T)\odot D^{-\nf{1}{2}}
\end{align}{}
\begin{align}
D = \nf{1}{(1+\lambda)^2} \left(\mathrm{I} \oslash \left(R \til{\Sigma}^{\nf{1}{2}} R^T - \lambda R \old{\Sigma}^{\nf{1}{2}}R^T\right)\right)^{-2}
\end{align}{}
\begin{align}
\Sigma = \nf{1}{(1+\lambda)^2} R^T\left(\mathrm{I} \oslash \left(R \til{\Sigma}^{\nf{1}{2}} R^T - \lambda R \old{\Sigma}^{\nf{1}{2}}R^T\right)\right)^{-2}R
\end{align}{}

\begin{align}
&z^2=x y \\
&\nf{\partial z^2}{\partial z} = \nf{\partial z^2}{\partial x}\nf{\partial x}{\partial z}
\end{align}

\subsubsection{Identities}

\begin{align}
    \left(\lambda \old{\Sigma}^{-1} - \til{\Sigma}^{-1} \right)^{-1} =& - \til{\Sigma} - \nf{1}{1+ \lambda\textrm{trace}\left(\old{\Sigma}^{-1}(- \til{\Sigma})\right)} (- \til{\Sigma})\lambda \old{\Sigma}^{-1}(- \til{\Sigma})
\end{align}

\begin{align}
    \ln|A| &= \textrm{trace}(\ln A)\\
    |e^{A}|&=e^{\textrm{trace}(A)}\\
    |A|&=e^{\textrm{trace}(\ln A)}\\
    |A|^{-1}&=1/|A|
\end{align}

\subsection{Variance 2}
Output of the convex layer: S, R: scaling and rotation matrix, which are used to correct the output of the model to comply with the constraints: 
\begin{align}
    &\Sigma = S R^T\til{\Sigma}R
\end{align}
\begin{align}
    &\argmin_{S, R} \textrm{trace}(R)+\textrm{trace}(S)\\
    &\st ~ \textrm{trace}(\old{\Sigma}^{-1} \Sigma) + k + \log|\old{\Sigma}| - \log|\Sigma| \leq \epsilon,
\end{align}

\subsection{Frobenius Norm}
\label{sec:Frobenius}
\begin{align}
	\mathcal{L}= |\til{\mu}-\mu|^2 + |\til{\Sigma}-\Sigma|^2_F + \lambda \left(|\old{\mu}-\mu|^2 + |\old{\Sigma}-\Sigma|^2_F-\epsilon\right)
\end{align}

\subsubsection{mean}
\begin{align}
    \nabla_{\mu} \mathcal{L}(\mu, \lambda) &= 2(\til{\mu}-\mu) + 2\lambda (\old{\mu}-\mu)\overset{!}{=} 0\\
    &\Longrightarrow \mu = \nf{\til{\mu} + \lambda\old{\mu}}{1+\lambda}
\end{align}

\begin{align}
&\mathcal{L}(\lambda)= \nf{\lambda}{1+\lambda}(\old{\mu}-\til{\mu})^2-\lambda\epsilon
\end{align}

\begin{align}
    \mathcal{L}(\lambda) &= \left|\til{\mu}-\left(\nf{\til{\mu}+\lambda\old{\mu}}{1+\lambda}\right) \right|^2 +\lambda\left| \old{\mu} - \nf{\til{\mu}+\lambda\old{\mu}}{1+\lambda}\right|^2 -\lambda\epsilon \\
    &= \left|\left(\nf{\til{\mu}(1+\lambda)-\til{\mu}-\lambda\old{\mu}}{1+\lambda}\right) \right|^2 +\lambda\left|  \nf{\old{\mu} (1+\lambda) -\til{\mu}-\lambda\old{\mu}}{1+\lambda}\right|^2 -\lambda\epsilon  \\
    &= \nf{\lambda^2}{(1+\lambda)^2} \left|\left(\til{\mu}-\old{\mu}\right) \right|^2 +\nf{\lambda}{(1+\lambda)^2}\left|\old{\mu} -\til{\mu}\right|^2 -\lambda\epsilon  \\
        &= \nf{\lambda(1+\lambda)}{(1+\lambda)^2} \left|\left(\til{\mu}-\old{\mu}\right) \right|^2 -\lambda\epsilon \\
        &= \nf{\lambda}{(1+\lambda)} \left|\left(\til{\mu}-\old{\mu}\right) \right|^2 -\lambda\epsilon
\end{align}

\begin{align}
    \partial_{\lambda}\mathcal{L}(\lambda) &= \left(\nf{1}{1+\lambda}-\nf{\lambda}{(1+\lambda)^2}\right)|\til{\mu}-\old{\mu}|^2-\epsilon\\
    &=\left(\nf{1}{(1+\lambda)^2}\right)|\til{\mu}-\old{\mu}|^2-\epsilon\\
    &\Longrightarrow \lambda^* = \nf{|\til{\mu}-\old{\mu}|}{\sqrt{\epsilon}}-1
\end{align}

\begin{align}
%    &\nabla_{\mu} L(\mu, \lambda) = 2\Sigma^{-1}(\mu - \til{\mu}) + 2\lambda \Sigma^{-1}(\mu - \old{\mu}) \overset{!}{=} 0\\
    &\Longrightarrow \mu^* = \old{\mu} +\nf{\sqrt{\epsilon}(\til{\mu}-\old{\mu})}{|\til{\mu}-\old{\mu}|}
\end{align}

\subsubsection{covariance}

\begin{align}
    \nabla_{S}\mathcal{L} &= 2 \left( \left(\til{\Sigma}-\Sigma \right) +\lambda \left(\old{\Sigma}-\Sigma\right)\right)\overset{!}{=} 0\\
    &\Longrightarrow \Sigma^* = \nf{1}{1+\lambda}\left( \til{\Sigma} +\lambda \old{\Sigma}\right)
\end{align}

\begin{align}
   \lambda^*&= \nf{|\til{\Sigma}-\old{\Sigma}|_F}{\sqrt{\epsilon}}-1 
\end{align}{}
 
\begin{align}
     \Sigma^*= \nf{\left(\til{\Sigma}+\left(\nf{|\til{\Sigma}-\old{\Sigma}|_F^2}{\epsilon} -\nf{1}{2}\right)\old{\Sigma}\right)}{\nf{1}{2}+\nf{|\til{\Sigma}-\old{\Sigma}|_F^2}{\epsilon}}
\end{align}

\subsection{Wasserstein}
The squared Wasserstein distance between two Gaussian distributions with parameters $\mu_1, \Sigma_1$ and $\mu_2, \Sigma_2$ is given by %\cite{DOWSON1982450}
\begin{align}
\label{eq:Wasserstein_distance}
        \mathcal{W}_2\left(\mathcal{N}\left(\mu_1, \Sigma_1\right), \mathcal{N}\left(\mu_1, \Sigma_1\right)\right)^2 = |\mu_1-\mu_2|^2 + \mathrm{tr}\left(\Sigma_1 + \Sigma_2 -2 \left(\Sigma_2^{\nicefrac{1}{2}}\Sigma_1\Sigma_2\nff\right)\nff \right) 
\end{align}{}
Using the Wasserstein distance both as objective and constraint in the constraint optimization problem we obtain the following Lagrangian:
\begin{align}
\label{eq:WassersteinLagrangian}
	\mathcal{L} &= |\til{\mu}-\mu|^2 + \mathrm{tr}\left(\til{\Sigma} + \Sigma -2 \left(\til{\Sigma}^{\nicefrac{1}{2}}\Sigma\til{\Sigma}\nff\right)\nff \right)\\
	&+ \lambda \left(|\old{\mu}-\mu|^2 +\mathrm{tr}\left(\old{\Sigma} + \Sigma -2 \left(\old{\Sigma}^{\nf{1}{2}}\Sigma\old{\Sigma}^{\nicefrac{1}{2}}\right)\nff\right)-\epsilon\right)
\end{align}

\subsubsection{mean}
The mean can be treated as above in \ref{sec:Frobenius}

\subsubsection{covariance}
Assuming that $\til{\Sigma}$ and $\Sigma$ as well as $\old{\Sigma}$ and 
 $\Sigma$ commute, the terms containing $\Sigma$ in  \ref{eq:WassersteinLagrangian} simplify to:
\begin{align}
    \mathcal{L} &= \mathrm{tr}\left(\til{\Sigma} + \Sigma -2 \til{\Sigma}^{\nicefrac{1}{2}}\Sigma\nf{1}{2} \right) + \lambda \left(\mathrm{tr}\left(\old{\Sigma} + \Sigma -2 \old{\Sigma}^{\nf{1}{2}}\Sigma^{\nicefrac{1}{2}}\right)-\epsilon\right)\\
    & = \mathrm{tr}\left(\til{\Sigma} + S^2 -2 \til{\Sigma}^{\nicefrac{1}{2}}S     \right) + \lambda \left(\mathrm{tr}\left(\old{\Sigma} +     S^2-2\old{\Sigma}\nf{1}{2}S\right)-\epsilon\right)
\end{align}
Here $S$ is the unique positive semi-definite root of the positive semi-definite matrix $\Sigma$, i.e. $S=\Sigma\nff$. 
Instead of optimizing the objective wrt $\Sigma$, we optimize wrt $S$ in order, which greatly simplifies the calculation. That is we solve
\begin{align}
    \nabla_{S}\mathcal{L} = (1+\lambda)2 S  -2 \left(\til{\Sigma}^{\nicefrac{1}{2}} + \lambda\old{\Sigma}\nff\right)\overset{!}{=} 0
\end{align}
for $S$, which leads us to:
\begin{align}
    S^* &= \nf{\til{\Sigma}\nff+\lambda\old{\Sigma}\nff}{1+\lambda}\\
    \Sigma^* &= \nf{\til{\Sigma}+\lambda^2\old{\Sigma}+2\lambda\til{\Sigma}\nff\old{\Sigma}\nff}{(1+\lambda)^2}\label{Sigma*}
\end{align}
This leads to the dual: 
\begin{align}
    \mathcal{L}(\lambda) & = \left( \tr{\til{\Sigma} +\old{\Sigma} - 2\til{\Sigma}\nff\old{\Sigma}\nff}\right)\cdot\left(\nf{\lambda}{1+\lambda}\right) - \lambda \epsilon 
\end{align}
and its derivative wrt. $\lambda$
\begin{align}
    \partial_{\lambda}\mathcal{L} =\left( \tr{\til{\Sigma} + \old{\Sigma} - 2\til{\Sigma}\nff\old{\Sigma}\nff}\right)\cdot\left(\nf{1}{(1+\lambda)^2}\right) -\epsilon
\end{align}
Now solving $\partial_{\lambda}\mathcal{L}\overset{!}{=} 0$
for $\lambda$ we arrive at
\begin{align}
    \lambda^*=\left(\nf{\tr{\til{\Sigma} +\old{\Sigma} - 2\til{\Sigma}\nff\old{\Sigma}\nff}}{\epsilon}\right)\nff -1
\end{align}
and plugging this into \ref{Sigma*} we obtain
\begin{align}
    \Sigma^* = \old{\Sigma} + \epsilon \nf{\til{\Sigma} + (1-2\eta)\old{\Sigma}+2(\eta-1)\til{\Sigma}\nff\old{\Sigma}\nff}{\tr{\til{\Sigma} +\old{\Sigma} - 2\til{\Sigma}\nff\old{\Sigma}\nff}}
\end{align}
where the abbreviation $\eta = \left(\nf{\tr{\til{\Sigma} +\old{\Sigma} - 2\til{\Sigma}\nff\old{\Sigma}\nff}}{\epsilon}\right)\nff$ was introduced.

\subsection{Wasserstein: Alternative derivation for non-commuting case}
In %\cite{Takatsu2008OnWG} 
the authors derive an expression for a geodesic between the two Gaussian distributions $\mathcal{N}(\mu_1, \Sigma_1)$ and $\mathcal{N}(\mu_2, \Sigma_2)$ in the space of Gaussian measures in $\mathrm{R^d}$.\\
Defining the symmetric positive definite matrix
\begin{align}
\label{eq:WMatrix}
W =\Sigma_2\nff\left(\Sigma_2\nff\Sigma_1\Sigma_2\nff \right)^{-\nicefrac{1}{2}}\Sigma_2\nff
\end{align}{}
as well as the expressions
\begin{align}
\label{eq:mu_t_Wasserstein}
l(t) &= (1-t)\mu_1 + t\mu_2\\
\label{eq:Sigma_t_Wasserstein}
W(t) &= ((1-t)\mathrm{I}+t\cdot W) \Sigma_1  ((1-t)\mathrm{I}+t\cdot W)
\end{align}{}
they show that the geodesic is given by
\begin{align}
\label{eq:geodesic}
	\left(\mathcal{N}(l(t), W(t))\right)_{t\in [0, 1]}
\end{align}

Starting from \ref{eq:geodesic} and using the expression for the squared Wasserstein distance between 
two Gaussian distribution \ref{eq:Wasserstein_distance}, we can obtain an equation for the parameter $t$.

\begin{align}
    \mathcal{W}_2\left(\mathcal{N}\left(\mu_1, \Sigma_1\right), \mathcal{N}\left(\mu_1, \Sigma_1\right)\right)^2 &\overset{!}{=}\epsilon^2 \\
    \label{eq:Wdist_N1N2}
    |\mu_1 - l(t)|^2 + \tr{\Sigma_1+ W(t) - 2\left( \Sigma_1\nff W(t)\Sigma_1\nff\right)\nff }&\overset{!}{=}\epsilon^2
\end{align}{}

For the calculation it is useful to first simplify the following terms:
\begin{align}
    \label{eq:trace_abbr1}
    \tr{W\Sigma_1}&=\tr{\Sigma_2\nff\left(\Sigma_2\nff\Sigma_1\Sigma_2\nff\right)^{-\nicefrac{1}{2}}\Sigma_2\nff\Sigma_1}=\tr{\left(\Sigma_2\nff\Sigma_1\Sigma_2\nff\right)^{\nicefrac{1}{2}}} \\
    \tr{W\Sigma_1W}&=\tr{\Sigma_2\nff\left(\Sigma_2\nff\Sigma_1\Sigma_2\nff\right)^{-\nicefrac{1}{2}}\left(\Sigma_2\nff\Sigma_1\Sigma_2\nff\right)\left(\Sigma_2\nff\Sigma_1\Sigma_2\nff\right)^{-\nicefrac{1}{2}}\Sigma_2\nff }\\
    & =\tr{\Sigma_2}\nonumber\\
    \label{eq:trace_abbr2}
    \tr{\Sigma_1\nff W(t)\nff} &= \tr{\Sigma_1(1-t)\mathrm{I}+t W} =(1-t)\tr{\Sigma_1}+t\cdot\tr{\left(\Sigma_2\nff\Sigma_1\Sigma_2\nff\right)^{\nicefrac{1}{2}}}
\end{align}
We now plug in the expression  \eqref{eq:mu_t_Wasserstein} and \eqref{eq:Sigma_t_Wasserstein} into \eqref{eq:Wdist_N1N2}:
\begin{align}
    \mathcal{W}_2^2 &=|\mu_1-(1-t)\mu_1 - t\mu_2|^2 + \tr{\Sigma_1} + \tr{((1-t)\mathrm{I}+t\cdot W) \Sigma_1  ((1-t)\mathrm{I}+t\cdot W)} \\
    & -2\tr{(1-t)\mathrm{I}+t\cdot W) \Sigma_1  ((1-t)\mathrm{I}+t\cdot W)\Sigma_1((1-t)\mathrm{I}+t\cdot W) \Sigma_1((1-t)\mathrm{I}+t\cdot W)}\nonumber\\
    &=t^2|\mu_1-\mu_2|^2 + \tr{\Sigma_1} + (1-t)^2 \tr{\Sigma_1}+ 2(1-t)t\cdot \tr{W\Sigma_1}\\ &
    + t^2 \tr{W\Sigma_1W} - 2\tr{\Sigma_1\nff W\nff}\overset{!}{=} \epsilon^2
\end{align}
We can now insert \eqref{eq:trace_abbr1} - \eqref{eq:trace_abbr2} to obtain:
\begin{align}
	\mathcal{W}_2^2 &=t^2|\mu_1-\mu_2|^2 +  t^2 \left(\tr{\Sigma_1} + \tr{\Sigma_2} - 2 \tr{\left(\Sigma_1\nff\Sigma_2\Sigma_1\nff\right)\nff} \right)\\
	&= t^2\left(|\mu_1-\mu_2|^2 + \tr{\Sigma_1+ \Sigma_2 - 2\left(\Sigma_1\nff\Sigma_2\Sigma_1\nff\right)\nff} \right) \overset{!}{=}\epsilon^2\\
	&\Rightarrow t = \frac{\epsilon}{\left(|\mu_1-\mu_2|^2 + \tr{\Sigma_1+ \Sigma_2 - 2\left(\Sigma_1\nff\Sigma_2\Sigma_1\nff\right)\nff} \right)\nff}
\end{align}

Now, setting $\mu_1=\old{\mu}, \Sigma_1=\old{\Sigma}, \mu_2=\til{\mu}, \Sigma_2=\til{\Sigma}$ and solving for t we obtain:

\begin{align}
    t = \frac{\epsilon}{\left(|\old{\mu} - \til{\mu}|^2 + \tr{\old{\Sigma} + \til{\Sigma} -2\left( \old{\Sigma}\nff \til{\Sigma} \old{\Sigma}\nff\right)\nff} \right)\nff}
\end{align}

\bibliographystyle{plain} % We choose the "plain" reference style
\bibliography{bibliography}

\end{document}
